# Supplementary material for: Fluctuated lattice-driven charge density wave far above the condensation temperature in kagome superconductor KV$_3$Sb$_5$
Source: arXiv:2504.16620 source file (2025-04-25)
Supplement: Supplementary file 1 [file KVS_Supplementary.pdf]

*Supplementary material for*

# Fluctuated lattice-driven charge density wave far above the condensation temperature in kagome superconductor $KV_3Sb_5$


Haoran Liu,[1] Shaofeng Duan,[1, 2, *] Xiangqi Liu,[3] Zhihua Liu,[1] Shichong Wang,[1] Lingxiao Gu,[1] Jiongyu Huang,[1] Wenxuan Yang,[1] Jianzhe Liu,[1] Dong Qian,[1, 4, 5] Yanfeng Guo,[3,6] and Wentao Zhang[2, 1, †]

[1]*Key Laboratory of Artificial Structures and Quantum Control (Ministry of Education),*

*School of Physics and Astronomy, Shanghai Jiao Tong University, Shanghai 200240, China*

[2]*Beijing National Laboratory for Condensed Matter Physics,*

*Institute of Physics, Chinese Academy of Sciences, Beijing 100190, China.*

[3]*School of Physical Science and Technology,*

*ShanghaiTech University, Shanghai 201210, China*

[4]*Tsung-Dao Lee Institute, Shanghai Jiao Tong University, Shanghai 200240, China*

[5]*Collaborative Innovation Center of Advanced Microstructures,*

*Nanjing University, Nanjing 210093, China*

[6]*ShanghaiTech Laboratory for Topological Physics, Shanghai 201210, China*


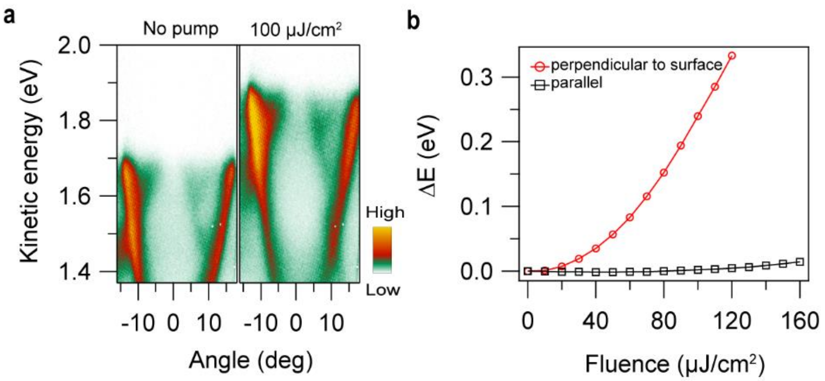


Supplementary Fig. 1. **Fluence-dependent band shift at $\overline{\Gamma}$ due to pump-induced space charge effect. a,** ARPES spectra at a delay time of -1 ps without a pump and with optical excitation at a fluence of 100 $\mu J/cm^2$. The light polarization is perpendicular to the sample surface. The spectrum exhibits a significant shift in kinetic energy after photoexcitation. **b**, Fluence-dependent band shift at -1 ps with the pump light polarized either perpendicular or parallel to the sample surface. The pump light polarized perpendicular to the surface induces a substantial overall energy shift in the spectrum, whereas the parallel polarized pump light causes only a minor change.


* sfduan@iphy.ac.cn

† wentaozhang@iphy.ac.cn

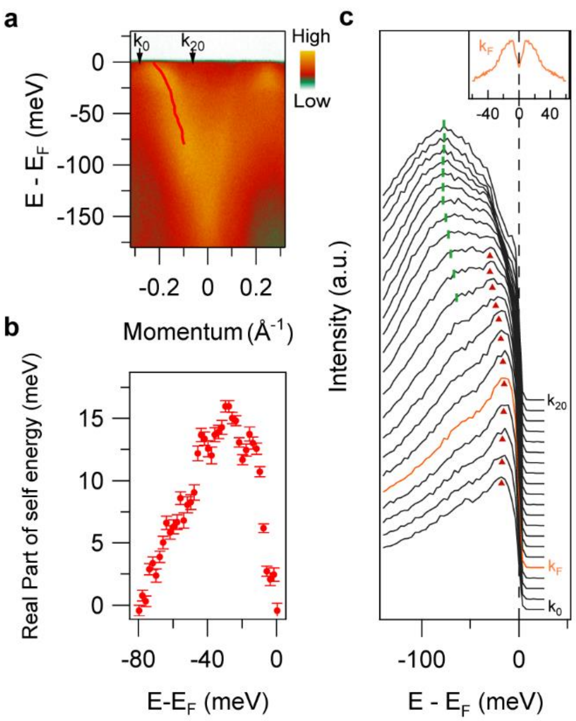


Supplementary Fig. 2. **Electron-phonon coupling in $KV_3Sb_5$. a,** ARPES spectrum along $\overline{\mathrm{K}}-\overline{\mathrm{M}}-\overline{\mathrm{K}}$, measured at 4.5 K. The dispersion of the $\gamma$ band is fitted from momentum distribution curves (MDCs). **b**, The real part of the electron self-energy. It is calculated by subtracting the linear bare band and shows a peak at approximately 30 meV. **c**, The corresponding energy distribution curves (EDCs) for the band structures in **a**. A peak-dip-hump structure can be observed, with peaks marked by triangles and the humps by bars. Inset: The symmetrized EDC at $k_F$ shows a CDW gap of about 10 meV.

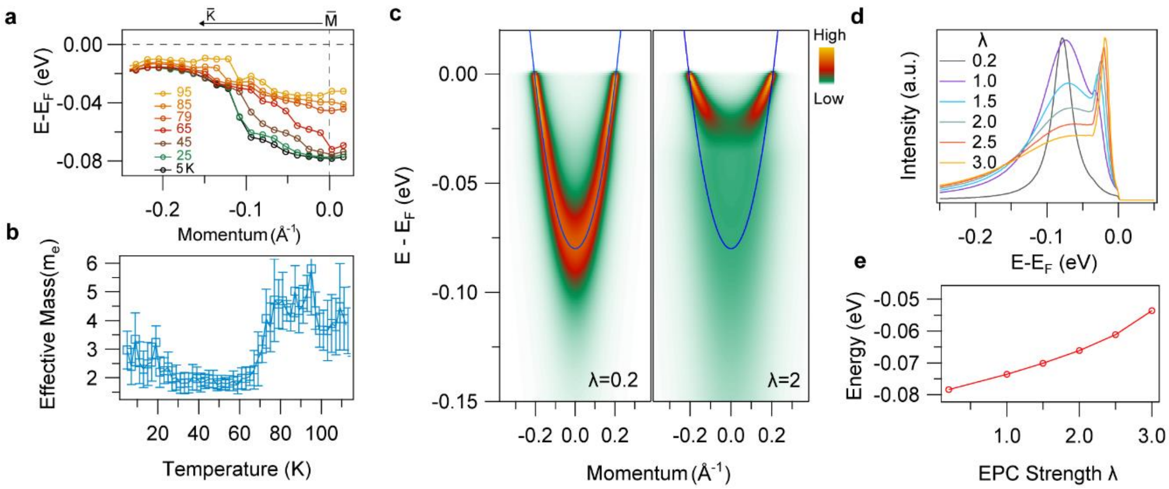


Supplementary Fig. 3. **Possible effective mass modification of the $\gamma$ band and influence of electron-phonon coupling on the band bottom.** **a**, Dispersion of the $\gamma$ band along $\overline{\mathrm{K}} - \overline{\mathrm{M}}$ direction at different temperatures. **b**, The effective mass of the $\gamma$ band fitted by a quadratic function. The effective mass shows a transition at $T_c$, as the band dispersion becomes flatter at $T_c$. **c**, The electronic band of the quadratic bare band (blue curve) with the electron-phonon coupling strengths $\lambda = 0.2$ and $\lambda = 2$, respectively. The Debye phonon with a peak at 30 meV is involved in the electron-phonon coupling. **d**, The EDCs at $k = 0$ with varied $\lambda$, showing the band bottom peak shifts towards the Fermi level as $\lambda$ increases. **e**, The $\lambda$ dependent band bottom shift.

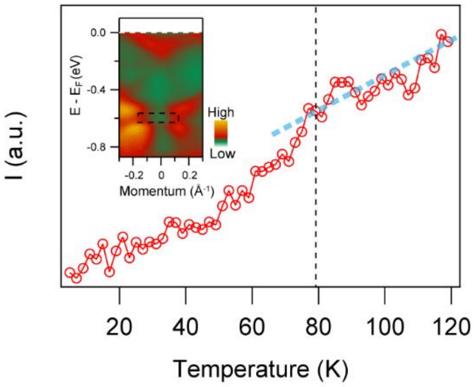


Supplementary Fig. 4. **Integrated intensity within the $\overline{\mathbf{M}}$ gap exhibits a transition near $\mathbf{T_c}$.** The light blue dashed lines indicate a transition at $T_c$. The black box in the inset denotes the integrated area.

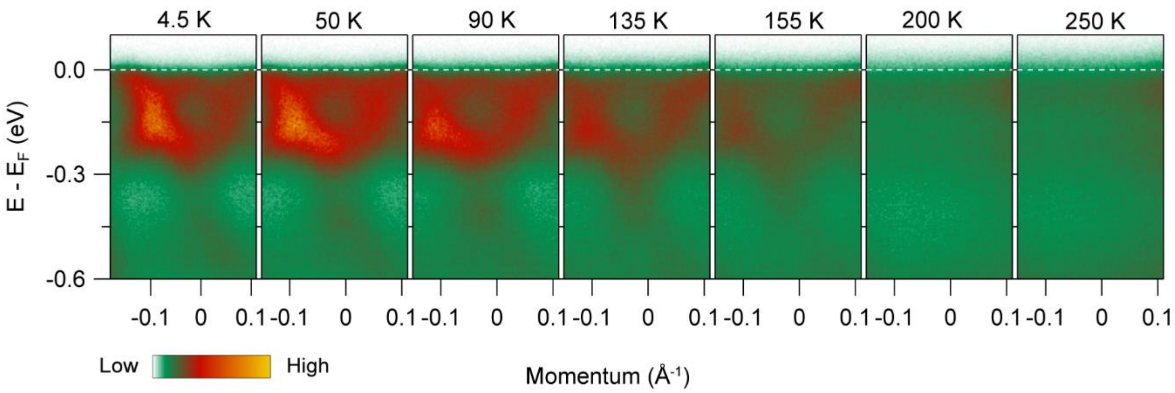


Supplementary Fig. 5. **The folded band measured on another sample during heating.** The folded band disappears at temperatures above 155 K.

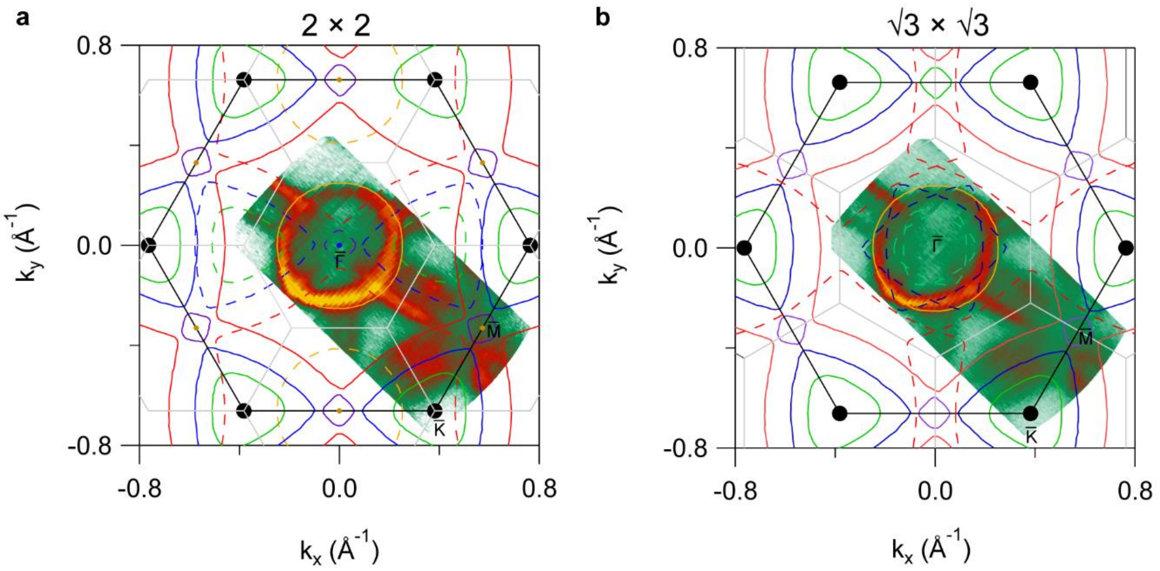


Supplementary Fig. 6. **Comparison of the folded bands between 2 × 2 and √3 × √3 reconstructions.** **a**, Fermi surface for the 2 × 2 reconstruction. **b**, Fermi surface for the √3 × √3 reconstruction. Dashed lines denote the folded bands. The 2 × 2 reconstructed bands align well with the Fermi surface mapping, whereas the √3 × √3 reconstructed bands do not.

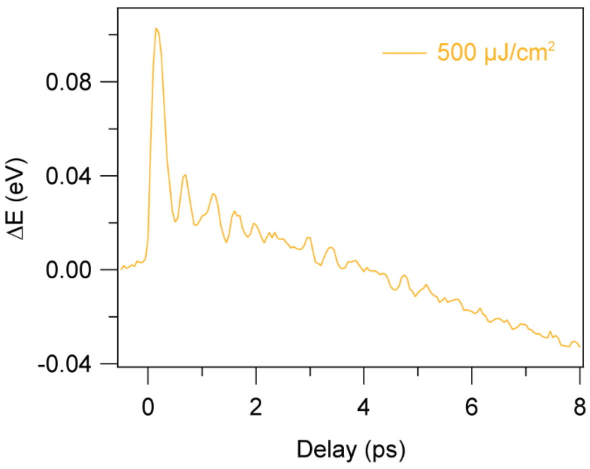


Supplementary Fig. 7. **Band shift near $\bar{\mathrm{M}}$ at a fluence of 500 $\mu$J/cm$^2$.** The shift is determined from the leading edge of the Fermi cut off. The rapid decay to negative values results from the pump induced space charge effect.

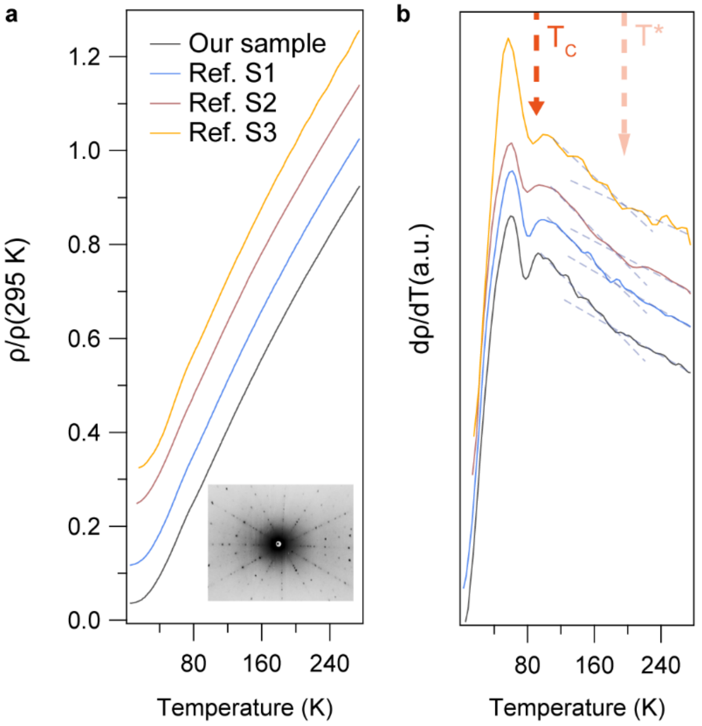


Supplementary Fig. 8. **Temperature-dependent in-plane resistance and its first derivative of $KV_3Sb_5$.** **a**, Temperature-dependent in-plane resistance of $KV_3Sb_5$ for our sample and the different references[S1–S3]. Inset: The Laue image of our sample. The clear Laue spots indicate that our sample is of good quality. **b**, First derivative of the resistance. The derivatives show a dip at $T_c$, signifying the CDW transition. The dashed lines represent the line fit of the derivative, revealing a weak dip between 160 and 200 K that suggests the onset of the CDW fluctuation at $T^*$. This dip arises from the sublinear resistivity of CDW kagome materials, which is closely related to the CDW properties[S4]. The data in **a** and **b** are offset for clarity.

**Supplementary Note 1. The pump-induced space charge effect**

The global shift of the band along the energy axis in $KV_3Sb_5$ is observed at a negative delay, as illustrated in Supplementary Fig. 1**a**. This shift depends on the polarization of the pump light, as shown in Supplementary Fig. 1**b**. A previous time- and angle- resolved photoemission experiment has identified a pump polarization-dependent space charge effect in $CsV_3Sb_5$[S5], which leads to the generation of a negative delay signal in the pump-probe photoemission spectra, analogous to observations in $KV_3Sb_5$. This negative delay signal is unlikely to arise from the photovoltage effect usually observed in the semiconductors and topological insulators[S6,S7], given the high conductivity of the $KV_3Sb_5$ and the observed pump polarization dependence. In our measurements, the pump polarization was oriented parallel to the sample surface to minimize the pump-induced space charge effect. The Fermi level of the fluence-dependent spectra was determined by fitting the negative delay spectra at each fluence.

**Supplementary Note 2. The effective mass modification and electron-phonon coupling of the γ band**

As the temperature increases, the $\gamma$ band becomes flatter (Supplementary Fig. 3**a**), indicating a transition in the effective mass at $T_c = 78$ K (Supplementary Fig. 3**b**). The effective mass transition suggests the electronic order transition at $T_c$. The dispersion of the $\gamma$ band shows a kink at approximately 30 meV (Supplementary Fig. 2), which is typically considered as a signature of electron-phonon coupling. At higher temperatures, this kink becomes less pronounced, raising the question of whether it affects the bottom of the $\gamma$ band. To investigate, we simulated the shift of the $\gamma$ band bottom as a function of electron-phonon coupling strength $\lambda$, following the procedure described in reference[S8]. As shown in Supplementary Fig. 3**c**, the quadratic bare band with the band bottom at 80 meV is only slightly modified with $\lambda = 0.2$. In contrast, the band is significantly altered and exhibits a prominent kink structure with $\lambda = 2$. The spectral weight and the peak position of the band bottom shift towards the Fermi level as the electron-phonon coupling strength increases (Supplementary Figs. 3**d** and 3**e**), indicating that a weaker electron-phonon coupling strength causes the band bottom to shift towards higher binding energies. This finding contradicts the observation that less apparent electron-phonon coupling at high temperatures coincides with the band bottom shifting towards the Fermi level (Supplementary Fig. 3**a**). Based on the simulation, we exclude the possibility that the shift of the band bottom is caused by the weakening of the electron-phonon coupling.

## Reference

S1. Ortiz, B. R. *et al.* Superconductivity in the Z2 kagome metal $KV_3Sb_5$. *Phys. Rev. Mater.* **5**, 034801 (2021).

S2. Luo, H. *et al.* Electronic nature of charge density wave and electron-phonon coupling in kagome superconductor $KV_3Sb_5$. *Nat. Commun.* **13**, 273 (2022).

S3. Uykur, E. *et al.* Optical detection of the density-wave instability in the kagome metal $KV_3Sb_5$. *npj Quantum Mater.* **7**, 16 (2022).

S4. Mozaffari, S. *et al.* Universal sublinear resistivity in vanadium kagome materials hosting charge density waves. *Phys. Rev. B* **110**, 035135 (2024).

S5. Azoury, D. *et al.* Direct observation of the collective modes of the charge density wave in the kagome metal $CsV_3Sb_5$. *Proc. Natl. Acad. Sci. U.S.A.* **120**, e2308588120 (2023).

S6. Yang, S.-L. *et al.* Electron propagation from a photo-excited surface: implications for time-resolved photoemission. *Appl. Phys. A* **116**, 85–90 (2014).

S7. Ciocys, S. *et al.* Tracking surface photovoltage dipole geometry in $Bi_2Se_3$ with time-resolved photoemission. *J. Stat. Mech.* **2019**, 104008 (2019).

S8. Sandvik, A. W., Scalapino, D. J. & Bickers, N. E. Effect of an electron-phonon interaction on the one-electron spectral weight of a *d*-wave superconductor. *Phys. Rev. B* **69**, 094523 (2004).
